# Supplementary material for: Can video generation replace cinematographers? Research on the cinematic language of generated video
Source: arXiv:2412.12223 source file (2025-03-28)
Supplement: Supplementary file 1 [file X_suppl.tex]

\setcounter{page}{1}
% \section{Rationale}
% \label{sec:rationale}
% % 
% Having the supplementary compiled together with the main paper means that:
% % 
% \begin{itemize}
% \item The supplementary can back-reference sections of the main paper, for example, we can refer to \ref{sec:intro};
% \item The main paper can forward reference sub-sections within the supplementary explicitly (e.g. referring to a particular experiment); 
% \item When submitted to arXiv, the supplementary will already included at the end of the paper.
% \end{itemize}
% % 
% To split the supplementary pages from the main paper, you can use \href{https://support.apple.com/en-ca/guide/preview/prvw11793/mac#:~:text=Delete%20a%20page%20from%20a,or%20choose%20Edit%20%3E%20Delete).}{Preview (on macOS)}, \href{https://www.adobe.com/acrobat/how-to/delete-pages-from-pdf.html#:~:text=Choose%20%E2%80%9CTools%E2%80%9D%20%3E%20%E2%80%9COrganize,or%20pages%20from%20the%20file.}{Adobe Acrobat} (on all OSs), as well as \href{https://superuser.com/questions/517986/is-it-possible-to-delete-some-pages-of-a-pdf-document}{command line tools}.
\section{Detailed Data Description}
To provide a more comprehensive introduction to the cinematography dataset, we further elaborate on the meanings of the 20 types of cinematic language in Section~\ref{apd:cinematic-language}.

\subsection{Cinematic2K Dataset.}
%要写出cinemadiff的和cameraclip的训练数据组成
\label{apd:Cinematic2K}
Cinematic2K consists of 20 categories based on shot framing, shot angle, and camera movement, with a total of 1945 instances of cinematic language data. A detailed description of these categories is provided in Section~\ref{apd:cinematic-language}. Each entry in the dataset includes a video, a description of the video, and a description of the cinematic language used. An example from Cinematic2K is shown in~\ref{fig:data_detailed}.

For CameraCLIP training, we divided the dataset into a training set with 1555 instances and a test set with 390 instances. During the training and validation stages, we compute the similarity between each video and its cinematic description. The cinematic description is structured as follows: "[video caption]." + "The shot type is:" + "[Cinematic Language] (shot framing, shot angle, camera movement)." For CameraDiff training, we define the video's category based on the "Main Cinematic Language." Additionally, to minimize the influence of irrelevant camera motions, we use "Typical Video" to select videos with typical cinematic features and "Interval" to annotate the precise cinematic type interval, ensuring data quality. Finally, for single-shot type learning, we use approximately 50 videos for each specific type.

\subsection{Meanings of 20 Types of Cinematic Language}
\label{apd:cinematic-language}
\begin{itemize}
    \item \textbf{Long Shot}: Shows the entire subject within its surroundings.
    \item \textbf{Medium Shot}: Captures the subject from the waist up, focusing on body language.
    \item \textbf{Close Up Shot}: Highlights a specific part of the subject, often the face, for detail.
    \item \textbf{Full Shot}: Frames the whole subject, providing context without much background.
    \item \textbf{Low Angle}: Camera positioned below the subject, making it appear powerful or imposing.
    \item \textbf{High Angle}: Camera positioned above the subject, making it seem smaller or vulnerable.
    \item \textbf{Bird Angle}: Overhead view, offering a comprehensive look at the scene from above.
    \item \textbf{Eye Level}: Camera is at the subject's eye height, creating a neutral perspective.
    \item \textbf{Dutch Angle}: Tilted camera angle, used to create tension or unease.
    \item \textbf{Rack Focus}: Shifts focus between subjects at different distances to guide viewer attention.
    \item \textbf{Panning Left}: Horizontal movement of the camera to the left, capturing a scene’s width.
    \item \textbf{Panning Right}: Horizontal movement of the camera to the right, capturing a scene’s width.
    \item \textbf{Tilt Up}: Vertical movement of the camera upwards, usually to reveal height.
    \item \textbf{Tilt Down}: Vertical movement of the camera downwards, often to show depth.
    \item \textbf{Dolly In}: Camera moves closer to the subject, creating an immersive effect.
    \item \textbf{Dolly Out}: Camera moves away from the subject, broadening the scene’s context.
    \item \textbf{Tracking Shot}: Camera follows the subject, maintaining focus while moving.
    \item \textbf{Zoom In}: Camera lens zooms in, bringing the subject closer without physical movement.
    \item \textbf{Zoom Out}: Camera lens zooms out, showing more of the surroundings.
    \item \textbf{Still}: The camera remains fixed, with no movement, offering a steady view.
\end{itemize}

\begin{figure*}[htbp]
    \centering
    \includegraphics[width=\textwidth]{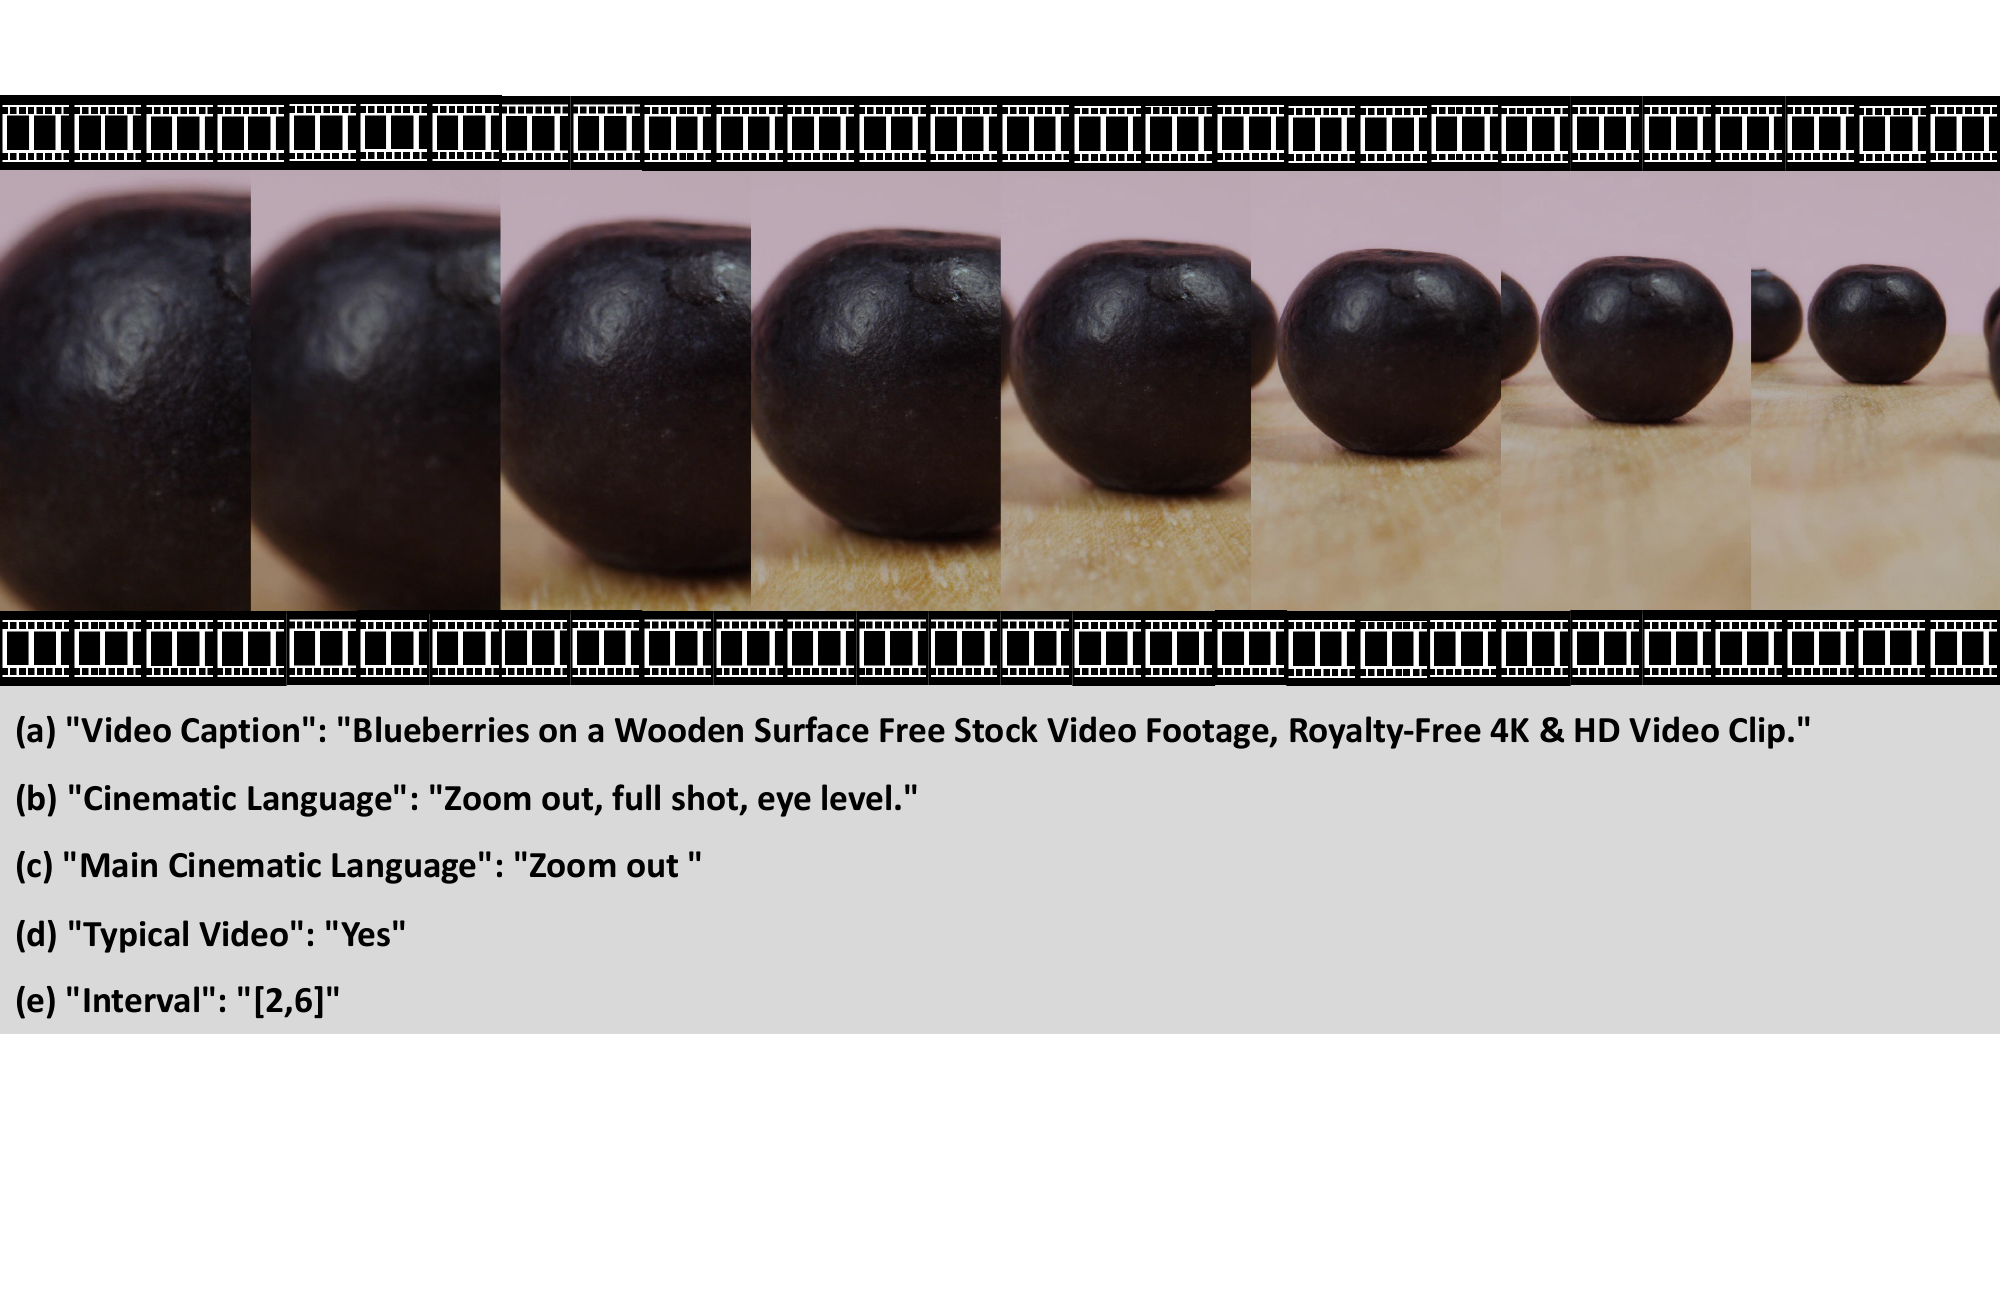}
    \caption{A sample from the Cinematic2K dataset. (a) "Video Caption" provides a textual description of the video. (b) "Cinematic Language" describes the cinematic language in the video. (c) "Main Cinematic Language" represents the primary shot type. (d) "Typical Video" denotes whether a video exhibits distinct cinematic features, with answers "Yes" or "No." (e) "Interval" annotates the precise cinematic type interval.}
    \label{fig:data_detailed}
\end{figure*}

\section{Detailed Settings}
\label{apd:experiment}
We provide the detailed description of the cameraCLIP's loss calculation in~\ref{apd:cameracliploss} and experimental settings in Section~\ref{apd:sec:cameraclip} for CameraCLIP and in Section~\ref{apd:sec:cliplora} for CLIPLoRA.

\subsection{CameraCLIP Loss Calculation}
\label{apd:cameracliploss}
We employ contrastive learning with the InFoNEC loss to align video and text features in a joint embedding space. To compute the similarity logits, we first apply \( L_2 \)-normalization to both the video features \( V \) and the text features \( T \), as follows:
\[
\hat{V} = \frac{V}{\|V\|_2}, \quad \hat{T} = \frac{T}{\|T\|_2},
\]
where \( \|\cdot\|_2 \) denotes the \( L_2 \)-norm. The similarity logits are then computed as:
\[
L_{\text{video}} = \frac{\hat{V} \cdot \hat{T}^\top}{\tau}, \quad L_{\text{text}} = L_{\text{video}}^\top,
\]
where \( \tau \) is the temperature parameter that controls the sharpness of the distribution. The cross-entropy loss for video-to-text and text-to-video matching is defined as:
\[
\mathcal{L}_{\text{video}} = \frac{1}{N} \sum_{i=1}^{N} -\log \frac{\exp(L_{\text{video}}(i,i))}{\sum_{j=1}^{N} \exp(L_{\text{video}}(i,j))},
\]
\[
\mathcal{L}_{\text{txt}} = \frac{1}{N} \sum_{i=1}^{N} -\log \frac{\exp(L_{\text{text}}(i,i))}{\sum_{j=1}^{N} \exp(L_{\text{text}}(i,j))}.
\]
The final loss function is the average of the video-to-text and text-to-video losses:
\[
\mathcal{L} = \frac{1}{2} (\mathcal{L}_{\text{video}} + \mathcal{L}_{\text{txt}}).
\]
This contrastive loss function effectively aligns the video and text modalities by maximizing the similarity between matching pairs and minimizing the similarity between non-matching pairs, thus ensuring accurate alignment of video and cinematic language text in our task.

\subsection{CameraCLIP Experimental Settings}
\label{apd:sec:cameraclip}
We trained the proposed CameraCLIP on a single NVIDIA A6000 Ada GPU (48GB). The specific training hyperparameters are detailed as follows:

\begin{itemize}
    \item \textbf{Batch size}: We set the batch size to 16.
    \item \textbf{Number of epochs}: The model was trained for 30 epochs.
    \item \textbf{Learning rate}: We used an initial learning rate of $2 \times 10^{-5}$, which was linearly increased during the first 10\% of training steps (warmup phase), followed by cosine annealing for the remaining steps. The final learning rate decayed to $10^{-6}$.
    \item \textbf{Optimizer}: We employed the AdamW optimizer~\cite{loshchilov2017decouple_adamw} with a weight decay of 0.2 to improve generalization.
    \item \textbf{Max length}: The maximum input length for text was set to 77 tokens, which is the default limit for the CLIP model.
    \item \textbf{Temperature parameter}: We set the temperature for the softmax operation to 0.01 to appropriately scale the logits during contrastive learning.
\end{itemize}
\subsection{CameraDiff Experimental Settings}
\label{apd:sec:cliplora}
This section outlines the experimental setup for training specific cinematic language patterns using LoRA and multi LoRA composition, as detailed in ~\ref{apd:cliplora_td}. Additionally, we describe the 26 text prompts used in this experiment for T2V generation in ~\ref{apd:prompt}.
\subsubsection{Training Details}
\label{apd:cliplora_td}
The training configuration for training specific cinematic language patterns using
LoRA~\cite{hulora} is based on the setting of AnimateDiff~\cite{guo2023animatediff}. We set both the LoRA rank and alpha to 32, as this configuration provides performance comparable to increasing the rank and alpha to 128 while requiring less training time. Each LoRA requires between 30 minutes and 1 hour of training on a single A100 with a learning rate of 1e-5 and a batch size of 4. The sample stride and number of frames are set to 4 and 16, respectively. Training is conducted for a maximum of 10 epochs per LoRA.
% , and the best epoch is selected using our proposed CameraCLIP method to prevent overfitting. 
% During training, we only employ the typical videos and sample within the typical range, as this approach yields better results than training with all the videos.

For the LoRA composition search in CLIPLoRA, we set the population size to 100 with 15 iterations, a mutation probability of 0.2, and a crossover probability of 0.5. The top 10\% of individuals are selected as elite candidates. The search is a discrete optimization process that determines which LoRA to use at each of the 50 steps in the denoising stage. A satisfactory result is typically achieved after three iterations, requiring approximately 200 minutes of computation on 8 Nvidia A100-80G GPUs. The majority of the time is spent generating the video over the 50 steps, using 26 prompts (see~\ref{apd:prompt} for more details) and evaluating the score with CameraCLIP. Note that CLIPLoRA is a 'search-once, inference-free' method, meaning that once the search is completed, the LoRA composition can be applied to all prompts without additional computational cost. During inference, our method operates identically to LoRA Switch, incurring no extra computational overhead.

\subsubsection{Prompts Used in Text-to-Video Generation}
\label{apd:prompt}

% \begin{tcolorbox}
\begin{itemize}
    \item Cricket still life with close up of ball and bat lying in the grass in front of stumps.
    \item A man is skiing.
    \item A rabbit is eating a watermelon on the table.
    \item A car is moving on the road.
    \item Bear playing guitar happily, snowing.
    \item Boy walking on the street.
    \item Ball And Bat Lying In Grass In Front Of Stumps.
    \item A black swan swims on the pond.
    \item A girl is riding a horse fast on grassland.
    \item A boy sits on a chair facing the sea.
    \item Two galleons moving in the wind at sunset.
    \item Cinematic photo melting pistachio ice cream dripping down the cone. 35mm photograph, film, bokeh.
    \item Large motion, surrounded by butterflies, a girl walks through a lush garden.
    \item An astronaut is waving his hands on the moon.
    \item A man cruises through the city on a motorcycle, feeling the adrenaline rush.
    \item A monkey eating a pizza in central park, GoPro film style
    \item A cyberpunk city street.
    \item A bird sits on a branch.
    \item A rabbit, forest, haze, halation, bloom, dramatic atmosphere, centered, rule of thirds, 200mm 1.4f macro shot.
    \item B\&W photo of a young man in black clothes, bald, face, body, high detailed skin, skin pores, coastline, overcast weather, wind, waves, 8k UHD, DSLR, soft lighting, high quality, film grain, Fujifilm XT3.
    \item Photo of coastline, rocks, storm weather, wind, waves, lightning, 8k UHD, DSLR, soft lighting, high quality, film grain, Fujifilm XT3.
    \item Night, B\&W photo of old house, post-apocalypse, forest, storm weather, wind, rocks, 8k UHD, DSLR, soft lighting, high quality, film grain.
    \item Pacific coast, Carmel by the sea ocean and waves.
    \item Robot dancing in Times Square.
    \item The Golden Temple in India.
    \item Flowers in Garden.
\end{itemize}
% \end{tcolorbox}
